# Supplementary material for: Ranking Clarifying Questions Based on Predicted User Engagement
Source: arXiv:2103.06192 source file (2021-04-01)
Supplement: Supplementary file 1 [file Appendix.tex]

\documentclass[../main.tex]{subfiles}

\begin{document}

\section{Appendix: Training implementation}
\subsection{Regression/Classification}\label{sec:parameters}
A \texttt{PyTorch} Multi-Layer Perceptron (MLP) is used for the regression \cite{Paszke_pytorch}. The input size is dependent on the representation used (TFIDF yields a larger vector). The Mean-Square Error (MSE) loss is used for training the regressor, and the Cross-Entropy (CE) loss is used for training the classifier. The optimal layer configuration and other hyperparameter settings are found by extensive hyperparameter tuning, performed on the balanced and impression filtered dataset and using regression. The optimal parameters are defined by the MSE-loss on the test set. Due to computational constraints, and given the similarity of the classification and regression model, the optimal parameters found for regression are also used for the classification model. In general, the model is quite robust to hyperparameter changes, but the following optimal values were found: Both the regression and classification model have two hidden layers of size $300$ and $32$ and make use of a \texttt{LeakyReLU} activation function with a negative slope of $0.02$ in every layer, as well as batch normalization ensure stable training and to combat overfitting. Dropout was included in the gridsearch but did not contribute to a better performing model. The \texttt{AmsGRAD} optimizer is used (SGD and Adam were also tested, with momentum), with a learning rate of $0.001$, and no weight decay.

\subsection{Ranker}
The RankNet model used in this paper uses a MLP, implemented in \texttt{PyTorch}, to predict the relative scores that determine the ranking \cite{Paszke_pytorch}. The input size is dependent on whether or not the predictions are included as features. In case they are, the input size is $5$, otherwise the input size is $4$. The model has two hidden layers of size $32$ and $16$. After every layer batch normalization is applied, followed by \texttt{LeakyReLU} as an activation function with a negative slope of $0.02$. The model is optimized using the \texttt{AmsGRAD} optimizer, with a learning rate of $0.001$ and a weight decay of $0.001$. These parameters are based on a limited gridsearch and heuristics.
\end{document}
